# Supplementary material for: Computational Study of pKa shift of Aspartate residue in Thioredoxin: Role of Configurational Sampling and Solvent Model
Source: arXiv:2211.13637 source file (2022-11-24)
Supplement: Supplementary file 1 [file SI_tidafed_paper.pdf]

# Supporting Information: Computational Study of p$K_a$ shift of Aspartate residue in Thioredoxin: Role of Configurational Sampling and Solvent Model

Shivani Verma and Nisanth N. Nair*

*Department of Chemistry, Indian Institute of Technology Kanpur, Kanpur - 208016, India*

E-mail: nnair@iitk.ac.in

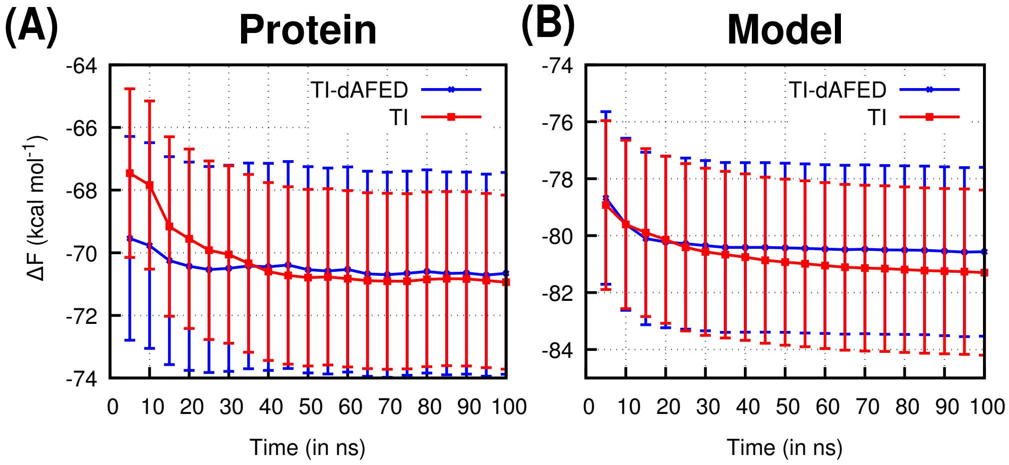


Figure 1: Convergence of free energy differences between protonated and deprotonated aspartic acid using TIP4P water model in (A) protein and (B) model. The blue and red colors depict the TI-dAFED and TI results, respectively.

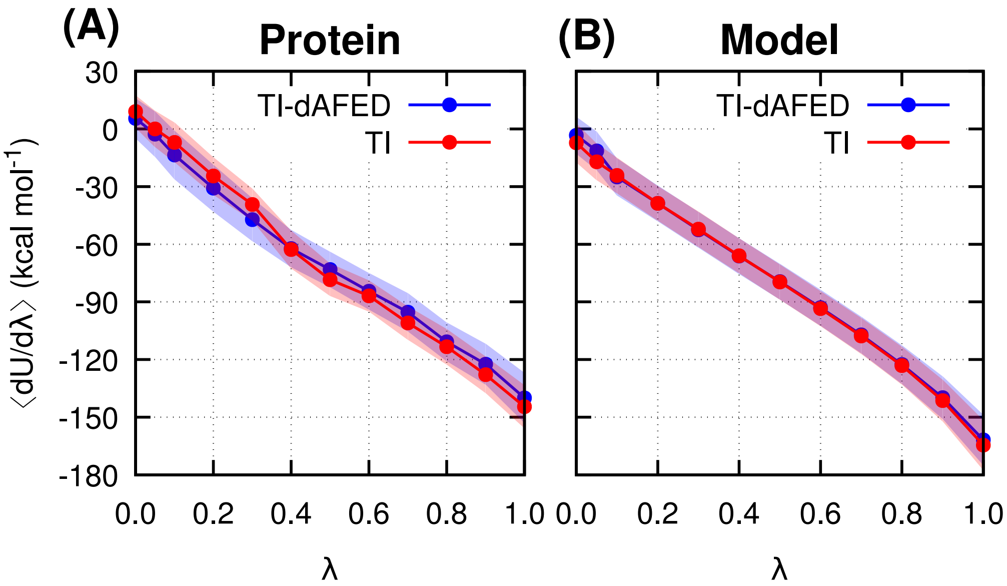


Figure 2: $\langle \mathrm{d}U/\mathrm{d}\lambda \rangle$ as a function of $\lambda$ for (A) protein and (B) model using the TIP4P water model. The blue and red colors depict the TI-dAFED and TI results, respectively.

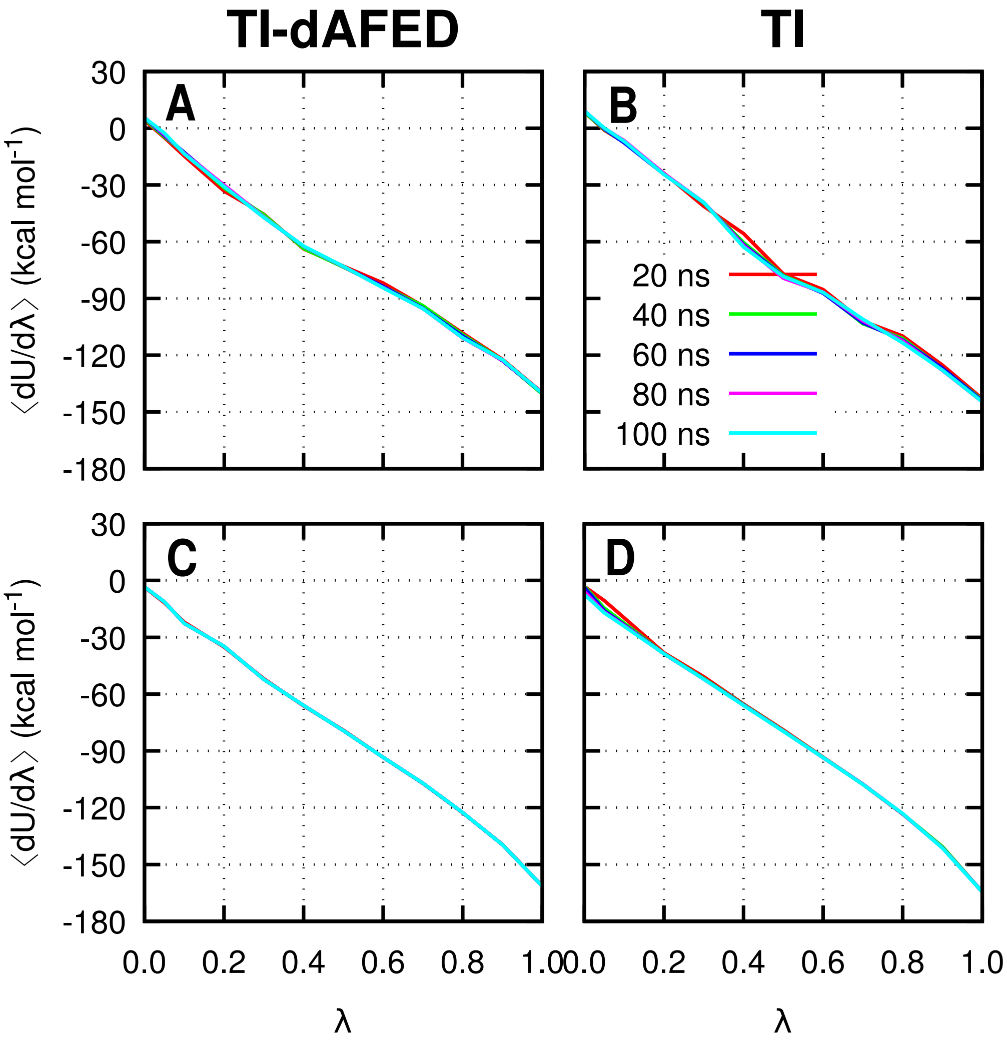


Figure 3: Convergence of $\langle \partial U/\partial \lambda \rangle$ as a function of $\lambda$ for (A) protein using TI-dAFED method, (B) protein using TI method, (C) model using TI-dAFED method and, (D) model using TI method. Here, the TIP4P water model is used.

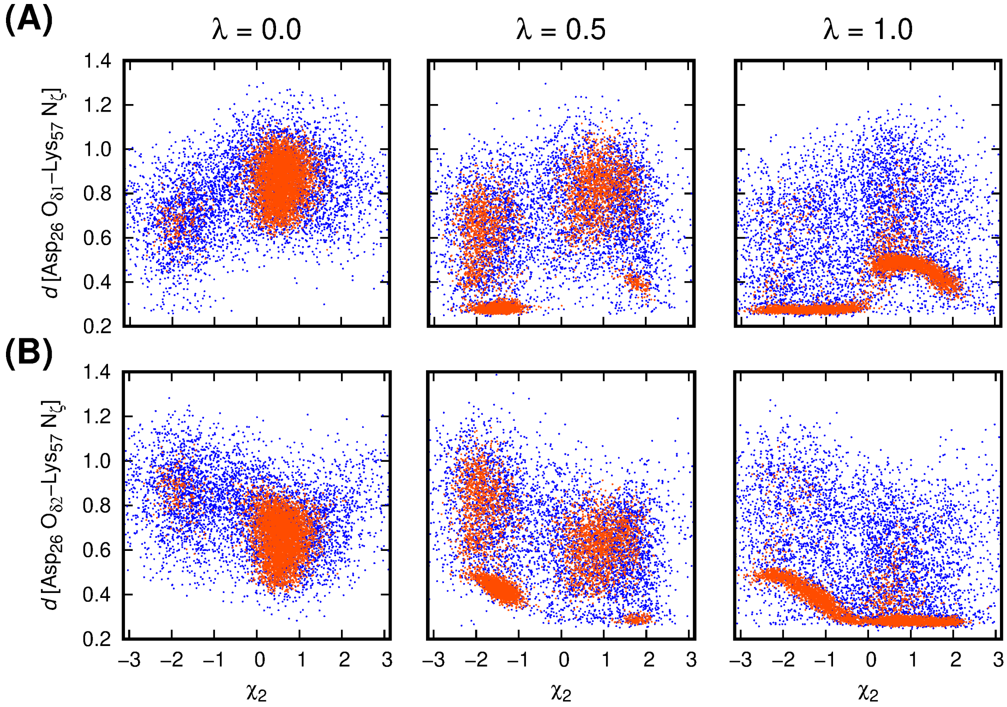


Figure 4: Scatter plot along $\chi_2$ and $d[\mathrm{Asp}_{26}\,\mathrm{O}_{\delta 1} - \mathrm{Lys}_{57}\,\mathrm{N}_{\zeta}]$ (A) and $\chi_2$ and $d[\mathrm{Asp}_{26}\,\mathrm{O}_{\delta 2} - \mathrm{Lys}_{57}\,\mathrm{N}_{\zeta}]$ coordinates (B) with TIP4P water model for $\lambda$ equals 0.0, 0.5, and 1.0. The blue and red colors depict the TI-dAFED and TI results, respectively.

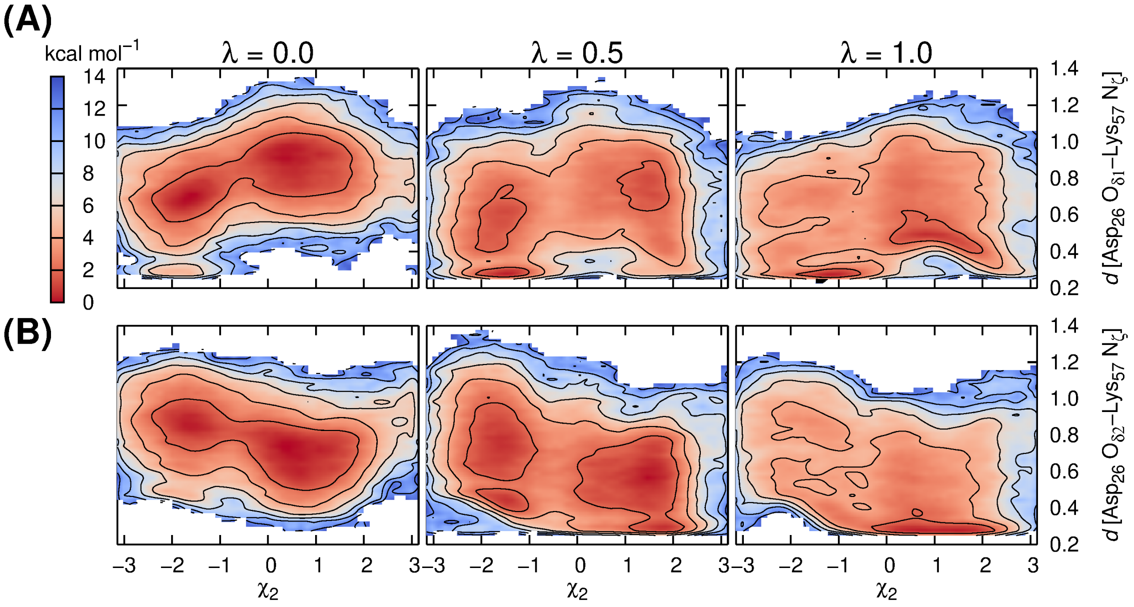


Figure 5: Free energy surface computed along $\chi_2$ and $d[\mathrm{Asp}_{26}\,\mathrm{O}_{\delta 1} - \mathrm{Lys}_{57}\,\mathrm{N}_{\zeta}]$ (A) and $\chi_2$ and $d[\mathrm{Asp}_{26}\,\mathrm{O}_{\delta 2} - \mathrm{Lys}_{57}\,\mathrm{N}_{\zeta}]$ (B) from the TI-dAFED simulations with TIP4P water model, for $\lambda$ equals 0.0, 0.5, and 1.0. Contours are drawn at 2 kcal mol$^{-1}$.
